# Supplementary material for: Nonparametric Bounds for Evaluating the Clinical Utility of Treatment Rules
Source: arXiv:2508.14653 ancillary file (2025-08-20)
Supplement: Supplementary file 1 [file supplement.pdf]

# Supplementary Materials for "Nonparameteric Bounds for Evaluating the Clinical Utility of Treatment Rules"

Johannes Hruza, Erin Gabriel, Arvid Sjölander,
Samir Bhatt, Michael Sachs

August 18, 2025

## 1 Proof of Theorem 1

*Proof.* Let $\mathcal{P}$ and $\mathcal{P}'$ be the sets of joint distributions compatible with $G$ and $G'$, respectively. Let $\boldsymbol{O}$ be the set of observed variables, which is the same in both models.

For a given $P_{\boldsymbol{V}} \in \mathcal{P}$, let $o(P_{\boldsymbol{V}})$ denote the observable marginal distribution of $\boldsymbol{O}$, which can be expressed as $o(P_{\boldsymbol{V}}) = \int P_{\boldsymbol{V}} d\boldsymbol{U}$. This defines the mapping $o : \mathcal{P} \to \mathcal{O}$ with $\mathcal{O} := \{o(P_{\boldsymbol{V}}) \mid P_{\boldsymbol{V}} \in \mathcal{P}\}$.

Similarly, for $G'$, let $o'(P_{\boldsymbol{V}})$ denote the observable marginal distribution of $\boldsymbol{O'}$, which defines the mapping $o' : \mathcal{P} \to \mathcal{O}'$ with $\mathcal{O}' := \{o'(P_{\boldsymbol{V}}) \mid P_{\boldsymbol{V}} \in \mathcal{P}\}$.

In $G'$, the merged variable $U = (U_1, U_2)$ represents the joint state space of $U_1$ and $U_2$. For any child $X$ of $U_1$ in $G$ with structural equation $X = g_X(pa(X), \epsilon_X)$ where $U_1 \in pa(X)$, the corresponding equation in $G'$ becomes $X = g_X(pa(X) \setminus \{U_1\}, P_1(U), \epsilon_X)$ with $U_1$ replaced by $P_1(U)$, where $P_1 : U \to U_1$ is the projection function that extracts the $U_1$ component from $U$. Similarly for children of $U_2$ or the combination of both.

Define a mapping $\varphi$ that transforms distributions in $G$ to distributions in $G'$ by replacing the separate distributions of $U_1$ and $U_2$ with their joint distribution:

$$\begin{aligned} \varphi \colon \mathcal{P} &\to \mathcal{P}' \\ P_{\boldsymbol{V}} &\mapsto P_{(\boldsymbol{V} \setminus \{U_1, U_2\}) \cup \{U\}} \end{aligned}$$

By construction, for any $P_{\boldsymbol{V}} \in \mathcal{P}$, the transformed distribution $\varphi(P_{\boldsymbol{V}})$ is compatible with $G'$, thus $\varphi(\mathcal{P}) \subseteq \mathcal{P}'$.

Furthermore, due to the nature of the transformation:

1. The causal parameter remains invariant: $\theta(\varphi(P_{\boldsymbol{V}})) = \theta(P_{\boldsymbol{V}})$ for all $P_{\boldsymbol{V}} \in \mathcal{P}$. This holds because the merged variable $U$ preserves all the causal relationships of $U_1$ and $U_2$.

2. The observable distributions remain the same: $o(P_{\boldsymbol{V}}) = o'(\varphi(P_{\boldsymbol{V}}))$ for all $P_{\boldsymbol{V}} \in \mathcal{P}$, where $o$ and $o'$ map distributions to their observable marginals in $G$ and $G'$, respectively.

Now, let $L'$ be a valid lower bound for $\theta$ in $G'$, meaning that for all $P_{\boldsymbol{V'}} \in \mathcal{P}'$:

$$L'(o'(P_{\boldsymbol{V'}})) \leq \theta(P_{\boldsymbol{V'}})$$

For any $P_{\boldsymbol{V}} \in \mathcal{P}$, we have:

$$\begin{aligned} L'(o(P_{\boldsymbol{V}})) &= L'(o'(\varphi(P_{\boldsymbol{V}}))) \\ &\leq \theta(\varphi(P_{\boldsymbol{V}})) \\ &= \theta(P_{\boldsymbol{V}}) \end{aligned}$$

Therefore, $L'$ is also a valid lower bound for $\theta$ in $G$. A similar argument applies for upper bounds. □

## 1.1 Ancestral graphs

In this section we will summarize the definitions and theorems used for the conditional bounds, which are known results and listed here for completeness, they are taken from Richardson and Spirtes (2002).

Conditioning on a variable in an existing DAGs is not closed, because after conditioning we can be left with a structure that does not satisfies the assumptions of a DAG. A simple example is $X \to S \leftarrow Y$ where conditioning on $S$ results in a structure that can not be described with a DAG.

An extension where such operations are allowed are mixed graphs.

**Definition 1** (graphical independence models)**.** *Let $G$ be a graph, $A$ separation criterion $C$ (for example d-separation) associates an independence model $I_C$ with graph $G$*

$$\langle X, Y \mid Z \rangle \in I_C(G) \Leftrightarrow X \text{ is separated from } Y \text{ by } Z \text{ in } G \text{ under criterion } C$$

**Definition 2** (mixed graphs)**.** *A mixed graph is a graph containing three types of edges, undirected, directed bidirected. Let $a, b$ be two vertices in $G$.*

$$\text{If} \left\{ \begin{array}{c} a - b \\ a \leftrightarrow b \\ a \to b \\ a \leftarrow b \end{array} \right\} \text{in } G \text{ then } a \text{ is a} \left\{ \begin{array}{l} \textit{neighbor} \\ \textit{spouse} \\ \textit{parent} \\ \textit{child} \end{array} \right\} \text{of } b \text{ and} \left\{ \begin{array}{c} a \in \mathrm{ne}_G(b) \\ a \in \mathrm{sp}_G(b) \\ a \in \mathrm{pa}_G(b) \\ a \in \mathrm{ch}_G(b) \end{array} \right\}.$$

**Definition 3** (ancestor, anterior)**.** *A path is sequence of edges for which the corresponding sequence of vertices contains no repetitions. A vertex $a$ is an ancestor of vertex $b$ if either there is a directed path $a \to \cdots \to b$ or $a = b$. A vertex $a$ is anterior to vertex $b$ if there is path from $a$ to $b$ with every edge either $-$ or $\to$.*

$$\begin{aligned} an(X) &= \{a \mid a \text{ is an ancestor of some } b \in X\} \\ ant(X) &= \{a \mid a \text{ is anterior to some } b \in X\} \end{aligned}$$

**Definition 4** (ancestral graph)**.** *An ancestral graph is a mixed graph which satisfies, $\forall a \in G$:*

*(i)* $a \notin ant(pa(a) \cup sp(a))$

*(ii)* *if* $ne(a) \neq \emptyset$ *then* $pa(a) \cup sp(a) = \emptyset$.

**Lemma 1.** *A DAG is an ancestral graph*

**Lemma 2.** *An ancestral graph has no directed cycles*

This implies that to show that an ancestral graph is a DAG one only has to show that it does not contain bidirect or undirect edges.

The idea of d-separation can be extended to ancestral graph under the name of m-separation

**Definition 5** (m-separation)**.** *A nonendpoint vertex $v$ on a path is a* ***collider on the path*** *if the edges preceding and succeeding $v$ on the path have an arrowhead at $v$, that is, $\to v \leftarrow$, $\leftrightarrow v \leftrightarrow$, $\to v \leftrightarrow$, $\leftrightarrow v \leftarrow$. A nonendpoint vertex $v$ on a path which is not a collider is a* ***noncollider on the path*** *on the path. A path between vertices $a$ and $b$ in an ancestral graph $\mathcal{G}$ is* ***m-connecting given a set*** *$Z$ (possibly empty), with $a, b \notin Z$, if:*

*(i) every noncollider on the path is not in $Z$, and*

*(ii) every collider on the path is in $an(Z)$.*

*If there is no path m-connecting $a$ and $b$ given $Z$, then $a$ and $b$ are said to be m-separated given $Z$. Sets $X$ and $Y$ are m-separated given $Z$, if for every pair $a, b$, with $a \in X$ and $b \in Y$, $a$ and $b$ are m-separated given $Z$ ($X, Y, Z$ are disjoint sets; $X, Y$ are nonempty). The independence model resulting from applying the m-separation criterion to $G$, is denoted by $I_m(G)$.*

**Theorem 1** (Theorem 4.18 in Richardson and Spirtes (2002)). *Let $G$ be an ancestral graph over vertices $V$ and $S \subseteq V$ (possibly be empty) a subset of vertices.*

*The indepencence model of $I_m(G)$ conditioning on $S$ is defined by:*

$$I_m(G)|^S := \{\langle X, Y \mid Z \rangle \mid \langle X, Y \mid Z \cup S \rangle \in I_m(G), (X \cup Y \cup Z) \cap S = \emptyset\}$$

*Define the transformation $(\cdot)|^S \colon G \mapsto G|^S$ is given by: Graph $G|^S$ has vertex set $V \setminus S$ and edges as follows:*

*For vertices $a, b \in V \setminus S$, s.t. $\forall Z$, with $Z \subseteq V \setminus (S \cup \{a, b\})$,*

$$\langle \{a\}, \{b\} \mid Z \cup S \rangle \notin \mathcal{I}_m(\mathcal{G})$$

*and*

$$\left\{ \begin{array}{c} a \in ant_G(\{b\} \cup S); b \in ant_G(\{a\} \cup S) \\ a \notin ant_G(\{b\} \cup S); b \in ant_G(\{a\} \cup S) \\ a \in ant_G(\{b\} \cup S); b \notin ant_G(\{a\} \cup S) \\ a \notin ant_G(\{b\} \cup S); b \notin ant_G(\{a\} \cup S) \end{array} \right\} \textit{then} \left\{ \begin{array}{c} a - b \\ a \leftarrow b \\ a \rightarrow b \\ a \leftrightarrow b \end{array} \right\} \textit{in } G|^S$$

.

*Then conditioning the graph $G$ on $S$ is the same as as applying the transformation, that is:*

$$I_M(G)|^S = I_m(G|^S)$$

Applying theorem 1 to the graph in figure 1 with $S = \{\boldsymbol{X}\}$ gives us the ancestral graphs in figure 3 respectively. In addition we notice that by lemma 2 and the fact that the transformation of the theorem does not introduce undirected or bidirectional edges that the resulting causal model is in fact a DAG.

## 1.2 Bounds for $\theta_f$ with 3 levels

Using linear programming methods (Balke and Pearl, 1997; Sachs et al., 2022) applied to the structure in Figure 2 a), we can derive sharp bounds for $\theta_f$ based on $P(A, Y, B)$. For the case where $A$ has three levels ($\mathcal{A} = \{a_0, a_1.a_2\}$) and $Y$ is binary, the sharp bounds on $\theta_f = P(Y(a_0) = 1, f(\boldsymbol{X}) = a_0) + P(Y(a_1) = 1, f(\boldsymbol{X}) = a_1) + P(Y(a_2) = 1, f(\boldsymbol{X}) = a_2)$ are given by:

$$\begin{aligned} L_R = 1 &- P(A=0,Y=0,f(\boldsymbol{X})=0) - P(A=1,Y=0,f(\boldsymbol{X})=0) - P(A=2,Y=0,f(\boldsymbol{X})=0) \\ &- P(A=1,Y=1,f(\boldsymbol{X})=0) - P(A=2,Y=1,f(\boldsymbol{X})=0) - P(A=0,Y=0,f(\boldsymbol{X})=1) \\ &- P(A=1,Y=0,f(\boldsymbol{X})=1) - P(A=2,Y=0,f(\boldsymbol{X})=1) - P(A=0,Y=1,f(\boldsymbol{X})=1) \\ &- P(A=2,Y=1,f(\boldsymbol{X})=1) - P(A=0,Y=0,f(\boldsymbol{X})=2) - P(A=1,Y=0,f(\boldsymbol{X})=2) \\ &- P(A=2,Y=0,f(\boldsymbol{X})=2) - P(A=0,Y=1,f(\boldsymbol{X})=2) - P(A=1,Y=1,f(\boldsymbol{X})=2) \\ U_R = 1 &- P(A=0,Y=0,f(\boldsymbol{X})=0) - P(A=1,Y=0,f(\boldsymbol{X})=1) - P(A=2,Y=0,f(\boldsymbol{X})=2) \end{aligned}$$

## 1.3 NPSEM for model with observed covariate $W$

The NPSEM for the non IV setting also illustrated by Figure 4 a) in the main text are given by:

$$\begin{aligned} \boldsymbol{u} &\sim P(\boldsymbol{u}) \\ \boldsymbol{x} &= h_X(\boldsymbol{u}, \epsilon_X) \\ w &= h_W(\boldsymbol{u}, \epsilon_W) \\ a &= h_A(\boldsymbol{u}, \boldsymbol{x}, w, \epsilon_A) \\ y &= h_Y(a, \boldsymbol{u}, \boldsymbol{x}, w, \epsilon_Y) \\ f(\boldsymbol{x}) & \quad \text{(deterministic in observed distribution)} \end{aligned}$$

### 1.4 Simulation

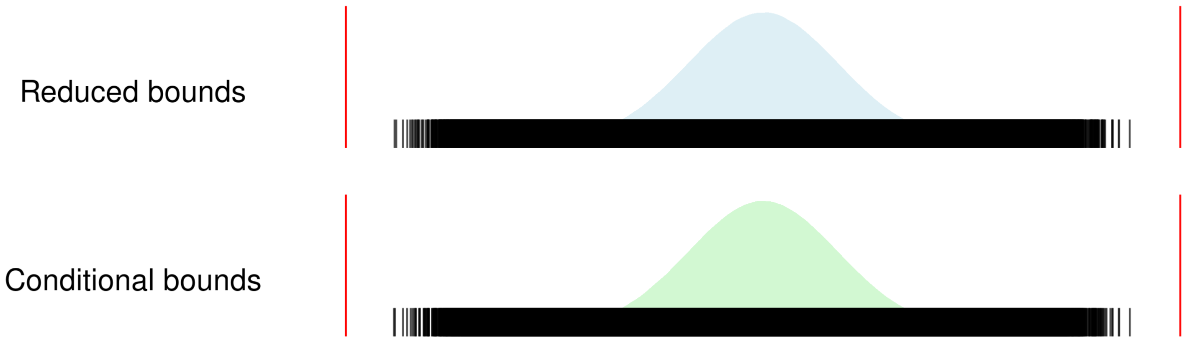


Figure 1: Simulation results of $10 \times 10^6$ runs of valid distributions and calculating the bounds based on the two proposed methods. The bounds (red lines) and the exact counterfactual value (black lines) are transformed such that they upper and lower bound coincide for all simulations.

The results have been transformed such that the upper and lower bounds coincide between all simulations. The exact counterfactual value, the lower bound $L$ and upper bound $U$ are transformed by $t$ given by $t(\cdot) = \frac{(\cdot)-L}{U-L}$. The black line is the exact counterfactual value and the red lines are the bounds. Due to the transformation a wider distribution implies that the exact value is closer to the bounds.

# References


Balke, A. and Pearl, J. (1997). Bounds on treatment effects from studies with imperfect compliance. *Journal of the American Statistical Association*, 92(439):1171–1176.

Richardson, T. and Spirtes, P. (2002). Ancestral graph markov models. *Ann. Stat.*, 30(4):962–1030.

Sachs, M. C., Jonzon, G., Sjölander, A., and Gabriel, E. E. (2022). A general method for deriving tight symbolic bounds on causal effects. *Journal of Computational and Graphical Statistics*, 32(2):567–576.
